# Supplementary material for: Medium Amplitude Parallel Superposition (MAPS) Rheology, Part 2: Experimental Protocols and Data Analysis
Source: arXiv:2006.09465 ancillary file (2020-06-16)
Supplement: Supplementary file 1 [file tutorial.pdf]

# Supplementary Material:
# Medium Amplitude Parallel Superposition (MAPS) Rheology
# Part 2: Experimental Protocols and Data Analysis

Kyle R. Lennon[1], Michela Geri[2], Gareth H. McKinley[2], and James W. Swan[1]

[1]*Department of Chemical Engineering, Massachusetts Institute of Technology, Cambridge, MA 02142*

[2]*Department of Mechanical Engineering, Massachusetts Institute of Technology, Cambridge, MA 02139*

## S1 Setting Up MITMAPS

The Supplemental Material for this work contains a version of the MITMAPS software package described in this work, as well as documentation, a license file, and this tutorial. Due to the large file sizes, the data files (titled "saos.txt" and "maps.txt") that were used to construct Figure 9 and Figures 11 through 16, which are referenced in this tutorial, are stored online at github.com/krlennon/mitmaps in the "Example Data" directory. Before installing the MITMAPS software, users should ensure that Python is installed with version $>$ 3.0.0. The version of the MITMAPS software included in this work is entirely Python-based, and its use will require at minimum modifications of the Python file titled "MITMAPS.py". Any updated versions of the software can be found at github.com/krlennon/mitmaps. We encourage interested users to contact the authors with any questions about the software.

The MITMAPS software package is composed of all files with the extension ".py" (i.e. "MITMAPS.py", "configuration.py", "mapsmodels.py", "mapsplot.py", "process.py", "mapsio.py", "mapssim.py", and "models.py"). To install the MITMAPS software, the user should simply download these files and place them in common directory, along with the files

"README.txt" and "COPYING.txt", which contain important information and documentation for the software ("README.txt") and the license for the software ("COPYING.txt"). We recommend that a new directory called "MITMAPS" is created to contain all of these files, which can be stored in a preferred location on a user's machine.

The files "saos.txt" and "maps.txt" contain the SAOS and MAPS data used to construct Figures 9, 11, 12, 13, and 14 of this work. These files should be downloaded from the online repository. In the below tutorial on creating those figures, we assume that the "saos.txt" file is stored in a sub-directory within the "MITMAPS" directory storing the ".py" files called "Examples", and that the "maps.txt" file is stored in a sub-directory within the "Examples" directory called "MAPS Data". The following file tree summarizes how the "MITMAPS" directory should be organized.

```
MITMAPS
 |__MITMAPS.py
 |__configuration.py
 |__mapsio.py
 |__mapsmodels.py
 |__mapsplot.py
 |__mapssim.py
 |__models.py
 |__process.py
 |__README.txt
 |__COPYING.txt
 |__Examples
     |__saos.txt
     |__MAPS Data
         |__maps.txt
```

Further documentation on the functionality of the MITMAPS software can be found in the README and at https://github.com/krlennon/mitmaps. In the following sections, we will briefly demonstrate how the software is used to generate Figures 9, 11, 12, 13, and 14 of this work, and how the software can be used to simulate MAPS data with simple differential constitutive models.

# S2 Processing MAPS Data

## S2.1 Data File Formats

The SAOS data used to generate Figure 9 of this work is contained entirely in the file "saos.txt". This data was collected using the Oscillatory Frequency Sweep mode in the TRIOS software provided by TA Instruments with the DHR-3 rheometer. In general, when a SAOS sweep is run for a material using the TRIOS software for use in the MITMAPS software, the resulting dataset should be exported to a plain text file. Further information on the format that this data file should take can be found in the README.

The MAPS data used to generate Figures 11, 12, 13, and 14 is contained entirely in the file "maps.txt". This data was collected using a series of Arbitrary Wave experiments. In each Arbitrary Wave experiment, the input stress waveform was specified with units of Pascals. In general, for MAPS sweeps run using the TRIOS software, the Arbitrary Wave experiments should be organized hierarchically based on 1) the input tone set $\{n_1, n_2, n_3\}$, 2) the amplitude $\sigma_0$, and 3) the fundamental frequency $\omega_0$, with the input signal defined by:

$$\sigma(t) = \sigma_0 \sum_{j=1}^{3} \sin(n_j \omega_0). \tag{S1}$$

In the case of the solution of wormlike micelles under study, which have a characteristic relaxation time of $\tau = 0.64s$ as measured by the SAOS sweep, for all fundamental frequencies studied it was sufficient to run each Arbitrary Wave experiment for approximately 10 periods with respect to the fundamental frequency $(10 \times (2\pi/\omega_0))$. This allows for the transient response to decay sufficiently, and leaves five full periods for analysis of the steady oscillatory state. This may have to be adjusted for different materials, and the data acquisition time should always be set to leave at least 5 periods with respect to the fundamental of approximately steady oscillatory data. The sampling rate should be set to a sufficiently high rate to reliably distinguish frequencies at least as high as the largest frequency under study.

| Experiment No. | $\{n_1, n_2, n_3\}$ | $\sigma_0$ (Pa) | $\omega_0$ (rad/s) | Acquisition Time (s) | Sampling Rate (1/s) |
|---|---|---|---|---|---|
| 1 | $\{5, 6, 9\}$ | 7 | 1.28 | 54 | 488 |
| 2 | | | 0.64 | 108 | 244 |
| 3 | | | 0.32 | 216 | 122 |
| 4 | | | 0.16 | 432 | 61 |
| 5 | | 3.5 | 1.28 | 54 | 488 |
| 6 | | | 0.64 | 108 | 244 |
| 7 | | | 0.32 | 216 | 122 |
| 8 | | | 0.16 | 432 | 61 |
| 9 | | 3.5 | 1.28 | 54 | 488 |
| 10 | | | 0.64 | 108 | 244 |
| 11 | | | 0.32 | 216 | 122 |
| 12 | | | 0.16 | 432 | 61 |
| 13 | $\{1, 4, 16\}$ | 7 | 1.28 | 54 | 488 |
| 14 | | | 0.64 | 108 | 244 |
| 15 | | | 0.32 | 216 | 122 |
| 16 | | | 0.16 | 432 | 61 |
| 17 | | 7 | 1.28 | 54 | 488 |
| 18 | | | 0.64 | 108 | 244 |
| 19 | | | 0.32 | 216 | 122 |
| 20 | | | 0.16 | 432 | 61 |
| 21 | | 7 | 1.28 | 54 | 488 |
| 22 | | | 0.64 | 108 | 244 |
| 23 | | | 0.32 | 216 | 122 |
| 24 | | | 0.16 | 432 | 61 |

Table S1: Order of Arbitrary Wave experiments entered into the TRIOS software to compose a MAPS frequency sweep.

However, higher sampling rates than necessary will increase the size of the data file, and therefore increase the processing time of the MITMAPS software, thus should be avoided. The ordering of experiments used to generate the data in the "maps.txt" file is presented in Table S1 along with the acquisition time and sampling rate used for each. The tone set, amplitude, and frequencies of experiments may be changed to suit a user's need, but it is important that the hierarchical ordering of the Arbitrary Wave experiments remain the same as in Table S1. The resulting data for all Amplitude Sweeps should be exported to one or more text files, with the filenames sorted alphanumerically in the same order of the experiment numbers. For more information regarding the required formats of data files, see

the README.

## S2.2 Using MITMAPS to Process MAPS Data

Here, we will describe how the MITMAPS software was used to generate Figures 9, 11, 12, 13, and 14 in this work using the data described above, contained in the "saos.txt" and "maps.txt" files. The software is structured such that the majority of the Python scripts comprise the back-end data processing, including file input, the mathematical data analysis described in this work, and plotting. The front-end of the software is contained primarily in the file "MITMAPS.py". In particular, we have highlighted a block of code containing all lines that need to be edited for minimal use of the software. Here, we will simply demonstrate how these lines should be edited to obtain the plots presented in Figures 9, 11, 12, 13, and 14 of this work. For a more detailed explanation of the back-end of the software, see the documentation within each file and in the README.

### S2.2.1 Plotting the Third Order Complex Compliance

To generate Figures 9, 11, and 12, the highlighted block of code should read as follows:

```
# Select the mode
mode = "experimental"

# Linear response
LR_file = "Examples/saos.txt"

# Experimental mode (either "stress" or "strain")
MAPS_control = "stress"

# MAPS response
MAPS_folder = "Examples/MAPS Data"
```

```
MAPS_tones = [[5,6,9],[1,4,16]]
MAPS_freqs = [1.28, 0.64, 0.32, 0.16]
sort_order = "amplitude"
plot_var = "J"

# Constitutive models
full_model = None
maps_models = [crm_J3]
extra_params = []

# Additional options
plotLR = True
gapLoading = False
outputTable = False
tssComp = False
```

The first line, `mode = "data"`, informs the software to run in experimental data mode (for more information on "data" vs. "simulation" mode see the README). The line `LR_file = "Examples/saos.txt"` sets the path to the file "saos.txt", assuming that the file is placed in a directory named "Examples" within the directory containing the MITMAPS software files. Note that the path here is valid for Unix-like systems, and will have to be adjusted for Windows systems. The second line `MAPS_control = "stress"` specifies that the experiments were conducted using stress control. The line `MAPS_folder = "Examples/MAPS Data"` sets the path to the directory containing the "maps.txt" file, in this case named "MAPS Data" and again contained in the "Experiments sub-directory. The following line, `MAPS_tones = [[5,6,9],[1,4,16]]`, indicates (in order) that the experiments in "saos.txt" represent MAPS frequency sweeps with the tone sets $\{n_1, n_2, n_3\} = \{5, 6, 9\}$ and $\{1, 4, 16\}$. The next line, `MAPS_freqs = [1.28, 0.64, 0.32, 0.16]` indicates that the frequencies (in order)

comprising the MAPS frequency sweep. The line `sort_order = "amplitude"` indicates that the second level in the hierarchical sorting of the Arbitrary Wave experiments is the amplitude of the input signal, $\sigma_0$. If another experiment is conducted which is sorted instead based on 1) the input tone set, 2) the frequency, and 3) the amplitude, this parameter can be changed to `"frequency"` (see the README). The line `plot_var = "J"` is used to specify that plots of the third order complex compliance are desired (as in Figures 11 and 12).

The next lines are used to specify a constitutive model(s) for plotting against the experimental MAPS data. The line `full_model = None` specifies that we do not wish to simulate any models (see the README for details on "simulation" mode). The line `models = [crm_J3]` specifies that the prediction for the third order complex compliance for the corotational Maxwell model should be plotted with the data. For a list of MAPS signatures for different constitutive models that can be plotted against data, see the file "mapsmodels.py". The line `extra_params = []` specifies that for the corotational Maxwell model, no parameters need be specified besides those regressed from the linear response. For models with adjustable nonlinear parameters (e.g. the Giesekus model), this variable should be set to a list of the values of all these adjustable parameters. The final four line indicate optional analyses that can be conduced based on the SAOS and MAPS data. The first of these lines, `plotLR = True`, specifies that we wish to plot the SAOS data to obtain the plots in Figure 9. The second, `gapLoading = False`, indicates that we do not wish to conduct gap loading limit analysis here (see Appendix C and the README for details). The line `outputTable = False` indicates that we do not wish to output the computed values of the MAPS response functions in tabular form, as a CSV file named "output.csv" contained in the same directory as the MITMAPS software files. The final line, `tssComp = False` indicates that we do not wish to conduct an analysis of whether the data obeys time-strain separability. For more information on these settings, see the README.

After making the above modifications to these lines, the MITMAPS script can be executed either within an IDE or directly from the shell using the command:

```
python3 MITMAPS.py
```

after which the plots that make up Figures 9, 11, and 12 should be displayed, along with Nyquist diagrams of the MAPS data and model predictions (which have not been included in this work). Note that the axes of these plots have been adjusted from their default settings in Figures 9, 11, and 12, and that axes labels have been added in a separate program.

#### S2.2.2 Plotting the Third Order Complex Viscosity

To recreate Figures 13 and 14, only two slight modifications need to be made to the "MITMAPS.py" file from the above configuration discussed above. Firstly, the line specifying the desired plotted variable should be changed to:

```
plot_var = "eta"
```

to specify that the third order complex viscosity should be displayed. Next, the line specifying the constitutive model solution should be changed to:

```
maps_models = [crm_eta3]
```

to specify that the third order complex viscosity prediction for the corotational Maxwell model should be displayed. Optionally, the user may also select that

```
plotLR = False
```

to suppress the linear response plots from being displayed again. By executing the script, the plots displayed in Figures 13 and 14 should be displayed, along with Nyquist diagrams that were not included in this work. Again, the axes of these plots have been modified from their defaults in this work, and axes labels have been added in a separate program.

## S3 Plotting Analytical MAPS Solutions

Using the MITMAPS software, it is also possible to plot the analytical solution for the MAPS response functions to different constitutive models, and to plot multiple solutions on

the same set of axes such as in Figures 15 and 16. Here we will provide a brief description of how to use the software to reproduce these figures. To do so, one must simply change to the "simulation" mode in the first line of the highlighted block:

```
# Select the mode
mode = "simulation"
```

To use the fit parameters from the linear response data, one should leave the line

```
# Linear response
LR_file = "Examples/saos.txt"
```

as is. The value of the variables `MAPS_control` and `MAPS_folder` are not relevant in "simulation" mode. The value of `MAPS_tones` still sets which input tone sets will be displayed in the plots, as in "experimental" mode. The maximum and minimum value of `MAPS_freqs` sets the range over which the model predictions are displayed. To generate Figures 15 and 16, we have left these lines as:

```
MAPS_tones = [[5,6,9],[1,4,16]]
MAPS_freqs = [1.28, 0.64, 0.32, 0.16]
```

though the setting `MAPS_freqs = [0.16, 1.28]` would have had the same effect. The value of `sort_order` is not relevant in "simulation" mode. To generate the plots of the third order complex compliance shown in Figures 15 and 16, we set

```
plot_var = "J"
```

The constitutive models are specified with the following lines:

```
# Constitutive models
full_model = None
maps_models = [crm_J3, giesekus_J3]
extra_params = [0.5]
```

The value of `full_model` should be set to `None` in "simulation" mode in order to avoid

plotting simulated MAPS data. To compare analytical MAPS solutions to simulated MAPS data for a constitutive model, this variable can be set to the name of any model in the file "models.py" (e.g. `full_model = crm` to simulate the corotational Maxwell model response to the MAPS tones given by `MAPS_tones` and frequencies given by `MAPS_freqs`). These numerical simulations can only be conducted in strain control, and are useful for numerically validating analytical solutions to constitutive models. See the README for more details on "simulation" mode for simulating MAPS data.

The line `maps_models = [crm_J3, giesekus_J3]` indicates that we would like to plot the predictions for the third order complex compliance from the corotational Maxwell model and Giesekus model. Any models found in the file "mapsmodels.py" can be used in this list, with up to two models plotted at once (for clarity). Note that the first model listed will be displayed with solid lines, and the second model with dashed lines. The line `extra_params = 0.5` specifies the value of the additional adjustable nonlinear parameter $\alpha = 0.5$ for the Giesekus model. If the value of `LR_file` is set to None, then `extra_params` should also contain the value of linear response parameters. For example, with no linear response file provided, and wishing to set $\eta_0 = 1$, $\tau = 1$, $\eta_\infty = 0$, and $\alpha = 0.5$, one would specify that `extra_params = [1,1,0,0.5]`. The remaining values for `plotLR`, `gapLoading`, `outputTable`, and `tssComp` should all be set to `False`. Executing the script described in this section will produce the plots shown in Figures 15 and 16, before additional modifications were made to the axes.
